# Supplementary material for: Staying True to Your Word: (How) Can Attention Become Explanation?
Source: arXiv:2005.09379 source file (2020-05-19)
Supplement: Supplementary file 1 [file raw_appendix.tex]

\begin{table*}[t]
\centering
\begin{tabular}{|c|c|c|c|c|c|c|c||c|}
\cline{3-8}
\multicolumn{2}{c}{} & \multicolumn{3}{|c|}{MLM} & \multicolumn{3}{|c||}{Base} & \multicolumn{1}{|c}{}\\
\cline{2-9}
\multicolumn{1}{c|}{} & $\alpha$ & $\uparrow$ Tr. & $\downarrow$ Unif. & $\downarrow$ Perm. & $\uparrow $Tr. & $\downarrow$ Unif. & $\downarrow$ Perm. & $\eta$ \\ \hline

\multirow{ 2}{*}{SST} & + & TBD & TBD & TBD & $0.842$ & $-0.028$ & $-0.050$ & \\
& $\bigcdot$ & TBD & TBD & TBD & $0.843$ & $-0.026$ & $-0.065$&  \\ \hline
\hline

\multirow{ 2}{*}{AGNEWS} & + & TBD & TBD & TBD & $0.959$ & $-0.023$ & $-0.039$ &  \\
& $\bigcdot$ & TBD & TBD & TBD & $0.959$ & $-0.023$ & $-0.038$ &  \\  \hline
\hline

\multirow{ 2}{*}{20NG} & + & TBD & TBD & TBD & $0.909$ & $-0.098$ & $-0.141$ &  \\
& $\bigcdot$ & TBD & TBD & TBD & $0.911$ & $-0.352$ & $-0.368$ &  \\  \hline
\hline

\multirow{ 2}{*}{IMDB} & + & TBD & TBD & TBD & $0.883$ & $-0.100$ & $-0.134$ &  \\
& $\bigcdot$ & TBD & TBD & TBD & $0.882$ & $-0.186$ & $-0.229$&  \\ \hline
\hline

\multirow{ 2}{*}{Anemia} & + & TBD & TBD & TBD & $0.924$ & $-0.216$ & $-0.224$ &  \\
& $\bigcdot$ & TBD & TBD & TBD & $0.927$ & $-0.102$ & $-0.144$ &  \\ \hline

\cline{3-8}
\multicolumn{2}{c}{} & \multicolumn{3}{|c|}{Tying=10} & \multicolumn{3}{|c||}{Tying=20} & \multicolumn{1}{|c}{}\\ \hline
\cline{2-9}

\multirow{ 2}{*}{SST} & + & $0.838$ & $-0.031$ & $-0.086$ & $0.827$ & $-0.067$ & $-0.154$ & \\
& $\bigcdot$ & $0.836$ & $-0.054$ & $-0.142$ & $0.843$ & $-0.031$ & $-0.139$  \\ \hline
\hline

\multirow{ 2}{*}{AGNEWS} & + & $0.954$ & $-0.035$ & $-0.158$ &$0.950$ & $-0.033$ & $-0.146$ &  \\
& $\bigcdot$ & $0.954$ & $-0.030$ & $-0.121$ & $0.954$ & $-0.030$ & $-0.122$ &  \\  \hline
\hline

\multirow{ 2}{*}{20NG} & + & $0.916$ & $-0.284$ & $-0.338$ & $0.914$ & $-0.397$ & $-0.432$ &  \\
& $\bigcdot$ & $0.910$ & $-0.287$ & $-0.340$ & $0.909$ & $-0.370$ & $-0.428$&  \\  \hline
\hline

\multirow{ 2}{*}{IMDB} & + & $0.874$ & $-0.552$ & $-0.448$ & $0.871$ & $-0.562$ & $-0.433$ &  \\
& $\bigcdot$ & $0.873$ & $-0.660$ & $-0.497$ & $0.872$ & $-0.577$ & $-0.453$ &  \\ \hline
\hline

\multirow{ 2}{*}{Anemia} & + & $0.920$ & $-0.163$ & $-0.210$ & $0.913$ & $-0.314$ & $-0.276$ &  \\
& $\bigcdot$ & $0.914$ & $-0.119$ & $-0.168$ & $0.910$ & nan & $-0.597$ &  \\ \hline

\cline{3-8}
\multicolumn{2}{c}{} & \multicolumn{3}{|c|}{Residual} & \multicolumn{3}{|c||}{Concat} & \multicolumn{1}{|c}{}\\\hline
\cline{2-9}

\multirow{ 2}{*}{SST} & + & $0.836$ & $-0.051$ & $-0.081$ & $0.837$ & $-0.036$ & $-0.062$ & \\
& $\bigcdot$ & $0.848$ & $-0.043$ & $-0.081$ & $0.850$ & $-0.046$ & $-0.086$ &  \\ \hline
\hline

\multirow{ 2}{*}{AGNEWS} & + & $0.958$ & $-0.017$ & $-0.034$ & $0.959$ & $-0.015$ & $-0.026$ &  \\
& $\bigcdot$ & $0.958$ & $-0.019$ & $-0.030$ & $0.961$ & $-0.019$ & $-0.030$ &  \\  \hline
\hline

\multirow{ 2}{*}{20NG} & + & $0.916$ & $-0.352$ & $-0.352$ & $0.913$ & $-0.250$ & $-0.282$ &  \\
& $\bigcdot$ & $0.921$ & $-0.126$ & $-0.146$ & $0.910$ & $-0.404$ & $-0.371$ &  \\  \hline
\hline

\multirow{ 2}{*}{IMDB} & + & $0.880$ & $-0.158$ & $-0.195$ & $0.883$ & $-0.102$ & $-0.140$ &  \\
& $\bigcdot$ & $0.881$ & $-0.232$ & $-0.262$ & $0.879$ & $-0.172$ & $-0.208$ &  \\ \hline
\hline

\multirow{ 2}{*}{Anemia} & + & $0.926$ & $-0.163$ & $-0.205$ & $0.928$ & $-0.193$ & $-0.222$ &  \\
& $\bigcdot$ & $0.923$ & $-0.097$ & $-0.133$ & $0.924$ & $-0.152$ & $-0.172$ &  \\ \hline

\end{tabular}
\caption{Robustness of classifiers with respect to attention perturbation}
\label{tab:results}
\end{table*}
